# Supplementary material for: Microsecond Consensus for Microsecond Applications
Source: arXiv:2010.06288 source file (2020-10-13)
Supplement: Supplementary file 1 [file extra.tex]

\subsection{Old/Extra}

\subsection{Holes}
\begin{invariant}[No holes up to FUO]
Let $p$ be a process and $f$ its FUO. Then $p$'s log contains a value at every index $i < f$.
\end{invariant}
\begin{proof}
Consider an index $i < f$ in $p$'s log. The FUO of $p$ could only have increased past $i$ at line~\ref{line:incrementFUO}, thus after $p$ succesfully wrote some value in all of its confirmed followers' logs (including its own) at line~\ref{line:writeAccept}. Furthermore, once a log slot contains a value, that slot never becomes empty again (Invariant~\ref{inv:values-not-erased}.
\end{proof}

\igor{Actually, the next invariant is not true without updateFollowers}

\Naama{Yeah. I think it would only hold if we have update followers whenever a new leader takes over, and we assume some sort of `confirmed followers', such that a new leader doesn't send values to $p$ unless it updated $p$'s log.}
\begin{invariant}[No holes]
For any process $p$, if $p$'s log contains a value at index $i$, then $p$'s log contains a value at every index $j$, $0 \le j \le i$.
\end{invariant}
\igor{But the following one should be:}
\Naama{Now with confirmed followers, I think the stronger invariant should hold. I think we can have these `no-holes' invariants after section 5 where we add the update-followers.}
\begin{invariant}[No holes between decided values]
If some value $v_i$ is decided at some index $i$, then for all $0 \le j \le i$, there exists some value $v_j$ such that $v_j$ is decided at $j$.
\end{invariant}

\begin{invariant} [Weak no holes.] \label{inv:weaknoholes}
Let $p$ be any process and $f$ be its FUO. Then, for every $0 \le i < f$, there exists some value $v_i \neq \bot$, such that $v_i$ is committed at $p$ at index $i$. 
\end{invariant}

\Naama{This depends on how we update the FUO. Assuming only leaders update the FUO by copying over everything between your FUO and theirs (either when taking over as leader or when you issue an `update' request, the following proof should work.}

\begin{proof}
We prove this by induction on the number of times FUO has been updated for any process in the execution.
Base: At the beginning of the execution, $FUO = 0$ for all processes, so the claim trivially holds.

Step: Assume that the claim holds in an execution in which the number of total FUO updates is at most $k$. Consider the $k+1$th time an FUO is updated, and let $p$ be the process whose FUO is updated at this time. Let the previous value of $p$'s FUO be $f$, and the new value be $f'$.

We consider two cases: either $p$ is the leader at the time of its $k+1$th FUO update, or it is a follower. If $p$ is the leader, then it updated its $FUO$ after writing some value $v_i \neq \bot$ at a quorum of processes at each index $f \leq i < f'$. \Naama{Allowing a leader to write to many slots by buffering or by having several outstanding, but only update its FUO upon completion of all.} This quorum of processes must include $p$ itself, since the quorum is determined by the first majority $p$ gets an acknowledgement from, and we always assume that $p$ receives an acknowledgement from itself in $0$ time. Thus, there is a value $v_i \neq \bot$ in each slot $i < f'$.
If $p$ was a follower, then its update of its FUO must have been done by the leader. Let the leader be $\ell$, and its FUO be $f_\ell$. Note that the only way in which $\ell$ can update $p$'s FUO is by copying over all of the values in its own log between $p$'s FUO $f$ and $\ell$'s FUO $f_\ell$ to $p$'s log, and then changing $p$'s FUO to $f_\ell$. Thus, $f' = f_\ell$. Note that by the induction hypothesis, the invariant holds at $\ell$; that is, in $\ell$'s log, all slots smaller than $f_\ell$ have non-$\bot$ values. Thus, $\ell$ copies over non-$\bot$ values in all indices $f \leq i < f'$ to $p$'s log, thereby preserving the invariant at $p$.
\end{proof}

\subsection{Other}
\begin{invariant}
At any given time, at most one process has write permission at a quorum.
\end{invariant}
\begin{proof}
Follows from: (1) any two quorums intersect and (2) at most one process has write permission on any given process at any given time.
\end{proof}

\begin{invariant}
For any quorum Q, the maximum minProposal in Q can only increase.
\end{invariant}
\Naama{Can't we say something stronger: that for all processes $p$, the minProposal of $p$ can only increase? That would imply this invariant, and might be easier to prove.}

\begin{invariant}
At any given time, for any index $i$, there can be at most one value $v$ decided at $i$.
\end{invariant}
\begin{proof}
Follows from the fact that any two quorums intersect and the fact that a process' log can contain at most one value at any index.
\end{proof}

\begin{definition}
A value $v$ decided at index $i$ is said to be decided \emph{with proposal number $num$} if $num$ is the lowest proposal number at index $i$ for any process that has $v$ at index $i$.
\end{definition}

\begin{invariant}
For any index $i$, if a value $v \neq \bot$ is made to be decided at $i$ with proposal number $prop_v$, then no other value can be written in index $i$ with a higher proposal number for any process. 
\end{invariant}

\begin{proof}[Rough sketch.]
%To write a value on any slot, you must first acquire write permission at a majority, because in line 11 you're writing the minProposal number and need to wait for a majority. \Naama{Need to specify behavior for if you get nacks.}
%If the previous leader managed to write its value on a majority before getting its permissions taken away...
\end{proof}

\begin{invariant}
For any index $i$, if some value $v$ becomes decided at $i$, then $v$ will remain decided at $i$ forever. 
\end{invariant}
\begin{proof}
%Assume the contrary and let $t_1, t_2$ be times such that $v$ becomes decided at $i$ at time $t_1$ and $t_2 > t_1$ is the earliest time when $v$ is no longer decided at $i$. Let $Q$ be a quorum such that, at time $t_1$, for every process $p$ in $Q$, $p$'s log contains $v$ at index $i$ ($Q$ must exist by the definition of decided value). Let $p_v$ be the leader that ensured that $v$ is written on all processes in $Q$ at time $t_1$.

%Since $v$ is not decided at time $t_2$, it must be the case that for some process $p$ in $Q$, $p$'s log does not contain $v$ at index $i$. Without loss of generality, let $p$ be the first process in $Q$ whose value at index $i$ changed to something other than $v$. Thus, some process $q$ must have overwritten $v$ in $p$'s log with some other value $v'$, at line~\ref{line:writeAccept}. Therefore, $q$ must have selected $v'$ as having the highest proposal number from a quorum $Q'$ at line~\ref{line:freshestValue}. Recall that any two quorums intersect at at least one process. Let $p' \in Q \cap Q'$. Since $p$ was the first process in $Q$ whose value at index $i$ changed to a value other than $v$, $p'$ must have had value $v$ at index $i$ when $q$ read it.

%Assume that $p'$'s value was not adopted by $q$. That is, the proposal number in $p'$'s $i$th slot was not the largest proposal number that $q$ observed for slot $i$ in $Q'$. Let $r \in Q'$ be the process whose $i$th slot had the largest proposal number. If $r$'s value at slot $i$ is $u \neq v$, then it must have been written by some leader $p_u$. Furthermore, 
\end{proof}
