# Supplementary material for: Microsecond Consensus for Microsecond Applications
Source: arXiv:2010.06288 source file (2020-10-13)
Supplement: Supplementary file 2 [file main.tex]

\documentclass[sigplan,10pt]{acmart}

%\newif\ifcamera
 % \cameratrue % comment out line for full version

%\usepackage{tonsmod}
%\usepackage[margin=1in]{geometry}
 %\usepackage[subtle]{savetrees}

%\usepackage{booktabs} % For formal tables
%\usepackage{enumitem}

\usepackage{latexsym,amsmath,amsfonts,amssymb,stmaryrd,mathtools}
\usepackage{amsthm}
\usepackage{listings, fancyvrb, multicol}

\lstset{basicstyle=\footnotesize\ttfamily, tabsize=2, escapeinside={@}{@}}
%\lstset{literate={<<}{{$\langle$}}1  {>>}{{$\rangle$}}1}
\lstset{literate={<<}{{$\langle$}}1  {>>}{{$\rangle$}}1}
\lstset{breaklines=true,
    postbreak=\mbox{\textcolor{red}{$\hookrightarrow$}\space}}
\lstset{language=C, morekeywords={CAS,commit,empty,job,taken,entry,GOTO,bool}}
\lstset{xleftmargin=5.0ex, numbers=left,numberstyle=\tiny, numberblanklines=false, frame=single, showstringspaces=false}
%\lstset{caption={\texttt{tuple} and \collect{} algorithms},captionpos=b,label={alg:collect}}
\makeatletter
\lst@Key{countblanklines}{true}[t]%
{\lstKV@SetIf{#1}\lst@ifcountblanklines}

\lst@AddToHook{OnEmptyLine}{%
	\lst@ifnumberblanklines\else%
	\lst@ifcountblanklines\else%
	\advance\c@lstnumber-\@ne\relax%
	\fi%
	\fi}
\makeatother

\title{Appendix: Proof of Correctness}
\begin{document}

\renewcommand\footnotetextcopyrightpermission[1]{}
\pagestyle{plain}
\settopmatter{printfolios=true}
\settopmatter{printacmref=false}
\author{}
\date{}

\appendix

\section{Proof of the Algorithm}\label{sec:proof}
\input{osdi/appendix/pseudocode}
\input{osdi/appendix/definitions}
\input{osdi/appendix/invariants}
\input{osdi/appendix/extensions}
\end{document}
